# Supplementary material for: Nuclear effects in neutrinoproduction of pions
Source: arXiv:1501.04306 ancillary file (2015-03-11)
Supplement: Supplementary file 1 [file ReadmeNUCL.pdf]

# Code for evaluation of $\nu$ DVMP cross-sections with account of nuclear effects

This package provides a library `libDVMP` which may be used for evaluation of the  $\nu$ DVMP cross-sections on nucleons and nuclei with various GPD models. Below are given short instructions how to compile and use it.

**Description:** This package provides a library `libDVMP` which may be used for evaluation of the  $\nu$ DVMP cross-sections in the framework discussed in the main paper. To evaluate the components of the differential cross-section  $d\sigma/dt d\ln x_B dQ^2 d\phi$  on a nucleon, it is necessary to call the function (declared in `headers/DVMP_XSection.h`)

```
int dvmp_XSection_dlnx_dt_dQ2_dphi(
    AbstractGPD fun, double* kins,
    process p, XSection* Sigma),
```

and for the same cross-section  $d\sigma/dt d\ln x_B dQ^2 d\phi$  on the nuclear target, call

```
int dvmp_XSection_Nucl_dlnx_dt_dQ2_dphi(
    AbstractGPD fun,
    NuclearStructureFunction funStruc,
    Nucleus Nucl, double* kins,
    process p, XSection* Sigma).
```

The first argument `fun` corresponds to a GPD function declared in `headers/GPDPDF.h`, the nuclear GPD function `funStruc` and nuclear structure `Nucl` are declared in `headers/Structure.h`; the array `kins` contains kinematic variables ordered as `kins[]={y,  $x_B$ ,  $t$ ,  $Q$ }`, where  $y = p \cdot q / p \cdot k$ ,  $x_B$  is a Bjorken variable,  $t$  is the momentum transfer squared,  $t = \Delta^2$ ,  $Q = \sqrt{-q^2}$ . The structure `process p` declared in `headers/phys.h` contains information on particles participating in the process and has the following elements<sup>1</sup>:

```
p.projectile  initial lepton ( $\nu$  or  $\bar{\nu}$ )
p.target      target ( $p$  for proton,
                 $n$  for neutron)
                For nuclei, use 10-digit codes
                introduced in section 42 of RPP [2]
                (so for example ground state carbon
                 $^{12}\text{C}$  in this scheme is 1000060120)
p.finalMeson  produced meson from
                octet of pseudogoldstones
                ( $\pi^{0,\pm}$ ,  $K_{L,S}$ ,  $K^\pm$  or  $\eta$ )
p.finalBaryon produced baryon from
                lowest octet ( $p$ ,  $n$ ,  $\Lambda$ ,  $\Sigma^{0,\pm}$ )
                For nuclei, use the same convention
                as for p.target
                For the incoherent process (with final
                nucleus breakup), use a code
                1009999990.
p.finalLepton produced lepton ( $\nu$ ,  $\bar{\nu}$ ,  $\mu^\pm$ )
```

If evaluation was successful, `SUCCESS` value is returned and elements of `Sigma` are set to the components of the unintegrated cross-section  $x_B d^4\sigma_k/dt dx_B dQ^2 d\phi$  according to the following table<sup>2</sup>:

|                            |                                                  |
|----------------------------|--------------------------------------------------|
| <code>Sigma.L</code>       | $\frac{d^4\sigma_L}{dt d\ln x_B dQ^2 d\phi}$     |
| <code>Sigma.T</code>       | $\frac{d^4\sigma_T}{dt d\ln x_B dQ^2 d\phi}$     |
| <code>Sigma.LT</code>      | $\frac{d^4\sigma_{LT}}{dt d\ln x_B dQ^2 d\phi}$  |
| <code>Sigma.TT</code>      | $\frac{d^4\sigma_{TT}}{dt d\ln x_B dQ^2 d\phi}$  |
| <code>Sigma.LPrimeT</code> | $\frac{d^4\sigma_{L'T}}{dt d\ln x_B dQ^2 d\phi}$ |
| <code>Sigma.TPrimeT</code> | $\frac{d^4\sigma_{T'T}}{dt d\ln x_B dQ^2 d\phi}$ |
| <code>Sigma.H.c[n]</code>  | $c_n$ -harmonics ( $n = 0, 1, 2$ )               |
| <code>Sigma.H.s[n]</code>  | $s_n$ -harmonics ( $n = 1, 2$ )                  |

Other possible return values are `PROCESS_NOT_FOUND` if process is unknown and `WRONG_KINEMATICS` if the cross-section in unphysical kinematics is called. In both cases components of `Sigma` are undefined. The GPD models needed for numerical evaluations are placed in separate library files in folder `libraries/`. With this package, we provide the Kroll-Goloskokov [1] GPD model (file `libKrollGoloskokovGPD11.so`) described in the text of the paper.

**Prerequisites:** To compile this code, You need to have `C` and `Fortran 77` compilers, `make` utility and a GNU scientific library (GSL) installed. The code was tested with `gcc v. 4.4` and `4.6` and Fortran compiler `gfortran` on Linux `x86-64` platform.

**Compilation:** To compile the code, You have to run `make all` in the code main directory. This will build the above-mentioned GPD library, the  $\nu$ DVMP library (`libDVMP.so`, `libDVMP.a`) and an example driving application `NuDVMP` (see source in `src/DVMP.c`) which shows how to load GPDs from corresponding libraries and evaluate the cross-section.

**Running:** After compilation, run from command-line

```
./NuDVMP --NeutrinoType NuMuBar
--Target Proton --Lepton MuPlus
--Meson PiZero --DeltaTr 0.2
--Baryon Neutron --lepton-fraction
0.5 --virtuality 2 --gpd-model
libraries/libKrollGoloskokovGPD11.so
```

or in a brief form<sup>3</sup>

<sup>2</sup> All the curves presented in the main paper correspond to a leading-twist cross-section  $d\sigma_L$

<sup>3</sup> Optionally, instead of particle names, PDG codes [2] of the particles can be used; only particles and processes mentioned in the text of the paper are supported.

<sup>1</sup> Values of all elements are PDG codes as given in Sec. 42 of [2].

```
./NuDVMP -N NuMuBar -T Proton
-L MuPlus -M PiZero -B
Neutron -y 0.5 -q 2 -d 0.2 -g
libraries/libKrollGoloskokovGPD11.so
```

This will evaluate the cross-section  $x_B d^4\sigma/dt dx_B dQ^2 d\phi$  for the process  $\bar{\nu}p \rightarrow \mu^+\pi^0 n$  as a function of  $x_B$  at virtuality  $Q = 2 \text{ GeV}$  and  $y = 0.5$ , with  $\Delta_\perp = 0.2 \text{ GeV}$  and using Kroll- Goloskokov GPD model. Optionally, instead of fixed  $\Delta_\perp$ , one can make evaluations at fixed  $t$  with `-t` option. If only leading twist results are needed, evaluations may be done faster with option `--use-twist3 no` or `--w n`.

For nuclear targets, use 10-digit codes from Sec. 42 of Review of Particle Physics [2]. For example,

```
NuDVMP_t -N NuMuBar -T 1000260560
-L MuPlus -M PiMinus -B
1000260560 -y 0.5 -q 2 -x 0.1 -g
libraries/libKrollGoloskokovGPD11.so
-S libraries/libNuclWalecka.so -w
n
```

will evaluate the  $t$ -dependence of the cross-section for the coherent process  $\bar{\nu}_\mu {}^{56}\text{Fe} \rightarrow \mu^+\pi^- {}^{56}\text{Fe}$  with gaussian smearing over the light-cone fraction in kinematics discussed above;

```
NuDVMP_t -N NuMuBar -T 1000260560
-L MuPlus -M PiMinus -B
1009999990 -y 0.5 -q 2 -x 0.1 -g
libraries/libKrollGoloskokovGPD11.so
-S libraries/libNuclWalecka.so -w
n
```

will evaluate the same  $t$ -dependence of the cross-section for the incoherent process  $\bar{\nu}_\mu {}^{56}\text{Fe} \rightarrow \mu^+\pi^- X$ . For nuclear targets evaluation is relatively slow due to integration over the light-cone fraction, for this reason we provide an MPI version of the code which can be compiled with `make bins_mpi`. The generated executable files will have a suffix `“_MPI”` and can be run with `mpirun`, using the same options as for single-CPU code. Please see file `obj/Makefile` for more details.

**Adding new GPD models:** In order to add a new GPD model, it is necessary to implement a function `ExternalGPD(double x, struct GPDkins k)`, where  $x$  is the quark light-cone fraction and `struct GPDkins` declared in `headers/GPDPDF.h` keeps all the information on the target kinematics.

The latter has the following elements:

<sup>4</sup> See declaration in `headers/Structure.h`

```
k.xi      skewness parameter  $\xi$ 
k.t        momentum transfer  $t = \Delta^2$ 
k.Q        Scale at which GPD is taken
k.flavour  GPD flavour
k.GPD_type Type of GPD, can be
           GPD_H ( $H$ ), GPD_E ( $E$ ), GPD_HTilde ( $\tilde{H}$ )
           GPD_ETilde ( $\tilde{E}$ ), GPD_T_H ( $H_T$ ), GPD_T_E ( $E_T$ ),
           GPD_T_HTilde ( $\tilde{H}_T$ ), GPD_T_ETilde ( $\tilde{E}_T$ ).
```

After successful compilation of the new GPD model `libNewGPD.so`, it can be used with `--gpd-model` option discussed above, without recompilation of other parts of the code.

**Adding new nuclear models:** In order to add a new nuclear model, You have to implement a function <sup>4</sup> `int NuclearStructure(double y, double xi, double t, Nucleus Nucl, double* Result)`, where  $y$  is the nucleon light-cone fraction,  $\xi$  is the skewness,  $t$  is the momentum transfer squared, `struct Nucleus` keeps information on a nucleus type and has the following elements:

```
Nucl.Lambda  Number of  $\Lambda$ 's, should be
              zero for normal nuclei
Nucl.A       Mass number
Nucl.Z       Atomic number
Nucl.isomerNumber Isomer number, 0 for
                  ground state nucleus
Nucl.mass    Mass of nucleus, in GeV
```

If evaluation succeeded, the library should return `SUCCESS` and set element of array `Result[3]` to values of  $\rho_p$ ,  $\rho_n$  and  $\rho_\Lambda$ -densities. Otherwise, may return `WRONG_KINEMATICS` if  $|t| < |t_{\min}(\xi)|$  or  $|\xi| > 1$ ; `PROCESS_NOT_FOUND` if a transition between initial and final nuclear states is not possible. After successful compilation of the the new nuclear model `libNewNuclearModel.so`, it can be used with `-S` or `--NuclearStructure` option discussed above, without recompilation of other parts of the code.

For more details, please see the header files in `headers/` directory. Each function has a Doxygen-style comments with detailed description. Corresponding `.c`-files are in `src/` directory.

## Acknowledgments

This work was supported in part by Fondecyt (Chile) grants No. 1140390 and 1140377.

[1] S. V. Goloskokov and P. Kroll, Eur. Phys. J. A **47**, 112 (2011) [arXiv:1106.4897 [hep-ph]].

[2] K.A. Olive *et al.* (Particle Data Group), Chin. Phys. C
